# Supplementary material for: Treatment Effect Bias from Sample Snooping: Blinding Outcomes is Neither Necessary nor Sufficient
Source: arXiv:2007.02514 ancillary file (2022-07-23)
Supplement: Supplementary file 1 [file blinding_supp_v4.0.pdf]

# Treatment effect bias from sample snooping: blinding outcomes is neither necessary nor sufficient (Supplementary Materials)

Aaron Fisher

Foundation Medicine Inc.; 150 Second St, Cambridge, MA 02141.  
afishe27@alumni.jh.edu.

April 20, 2021

## Contents

|          |                                                                                |           |
|----------|--------------------------------------------------------------------------------|-----------|
| <b>A</b> | <b>Introduction</b>                                                            | <b>2</b>  |
| <b>B</b> | <b>Absolute bias from arbitrarily strong overfitting</b>                       | <b>2</b>  |
| <b>C</b> | <b>Additional simulation results</b>                                           | <b>3</b>  |
| <b>D</b> | <b>Helpful relationships used in proofs</b>                                    | <b>4</b>  |
| <b>E</b> | <b>Proof of Theorem 1 and its corollaries</b>                                  | <b>6</b>  |
| E.1      | Proof of Theorem 1 . . . . .                                                   | 6         |
| E.1.1    | Preliminaries: mediation and omitted variables in linear regression . .        | 6         |
| E.1.2    | Showing Eq (4) . . . . .                                                       | 9         |
| E.1.3    | Supplemental details on spherical distributions . . . . .                      | 12        |
| E.2      | Proof of Corollary 6 . . . . .                                                 | 14        |
| <b>F</b> | <b>Proofs for Theorem 2 and associated results</b>                             | <b>14</b> |
| F.1      | Proof of Theorem 2 . . . . .                                                   | 14        |
| F.2      | Proof of Remark 10 . . . . .                                                   | 16        |
| F.3      | Proof of Corollaries 4 & 5 . . . . .                                           | 17        |
| <b>G</b> | <b>Proof of Remark 8</b>                                                       | <b>18</b> |
| <b>H</b> | <b>Proof of Theorem B.1</b>                                                    | <b>18</b> |
| H.1      | Preliminaries: worst-case features in unblinded and blinded settings . . . . . | 19        |
| H.1.1    | Proof of Lemmas H.2 & H.4 . . . . .                                            | 20        |
| H.2      | Proof of Eq (B.1) . . . . .                                                    | 21        |

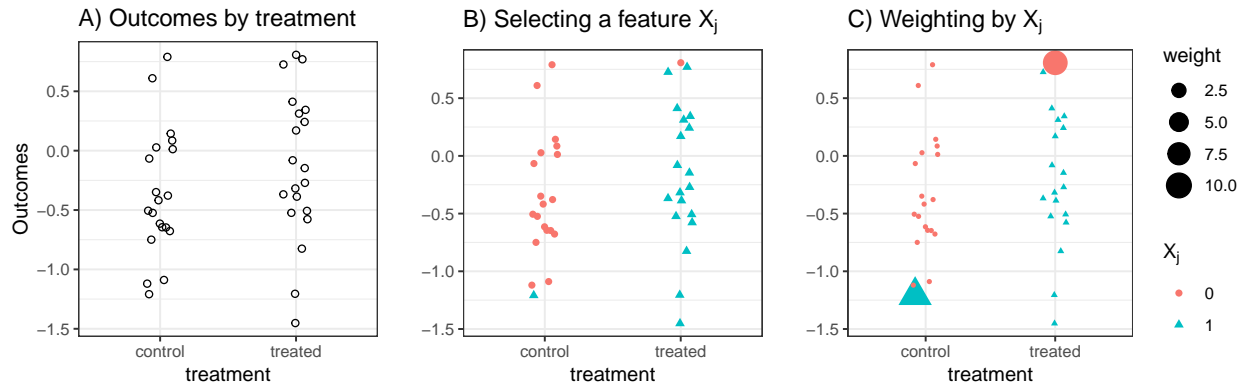

Figure B.1: Worst-case weighting – Panel (A) shows an example of synthetic data. Panel (B) colors each observation by a worst-case feature  $\mathbf{X}_j$  (see Section H.1). Panel (C) shows the weighted data set, using inverse propensity score weights based on  $\mathbf{X}_j$ .

H.3 Proof of Eq (B.2) . . . . . 22

## A Introduction

To disambiguate references to the main text from cross-references within this supplement, we use letters when referencing sections, figures and equations within this document (for example, Eq (B.1) in Section B of this document), and numbers when referencing the main text (for example, Eq (1) in Section 1.1 of the main text).

## B Absolute bias from arbitrarily strong overfitting

Section 2 focuses on the *relative* bias of blinded and snooping analysts. In this section, we study how bad the bias of either analyst can be on an *absolute* scale. Specifically, we study a worst-case scenario where analysts can overfit using arbitrarily complex categorical features. In this way, we can upper bound the absolute bias as the number of feature candidates  $p \rightarrow \infty$ . We find that the upper bound can indeed be severe.

Suppose that the features available for adjustment,  $\mathbf{X}_1, \dots, \mathbf{X}_p$ , are all categorical, and  $d = d_{\text{IPW}}$ . For this setting, we show in Section H.1 that any feature adjustment achieving large bias will do so by upweighting the extremes of the sample. An illustration of this kind of upweighting is shown in Figure B.1, in which the true treatment effect is zero, but an artificial effect can be produced by upweighting high outcomes on treatment and upweighting low outcomes on control. Here, the bias produced by conditioning on  $\mathbf{X}_j$  is dramatic.

The problem is only worsened in larger samples, where the sample extremes tend to stretch further and further apart. We formalize this in the theorem below.

**Theorem B.1.** (*Worst-case absolute bias*) Suppose that the following conditions hold.

1. (*Discrete covariates*) The random variables  $\mathbf{X}_1, \dots, \mathbf{X}_p$  are discrete.

2. (Constant effect)  $\tilde{Y}_i^{treat} = \tilde{Y}_i^{control} + \Delta$ , that is, the individual treatment effect takes the form of a constant (possibly null) shift.
3. (No confounders)  $P(\tilde{Y}^{treat}, \mathbf{X} | \mathbf{A} = 1) = P(\tilde{Y}^{treat}, \mathbf{X})$  and  $P(\tilde{Y}^{control}, \mathbf{X} | \mathbf{A} = 0) = P(\tilde{Y}^{control}, \mathbf{X})$ .
4. (Fixed assignment)  $n$  is an even number no less than 4; and  $A_i$  is deterministic, with  $A_i = 0$  for  $i \leq n/2$  and  $A_i = 1$  for  $i > n/2$ .
5. (IPW estimators) the estimator function  $d$  is equal to  $d_{IPW}$ .

Under these conditions,

$$E\left(\hat{\Delta}_{snoop}(\mathbf{X}, \mathbf{Y})\right) - \Delta \leq E\left(\max_{\{i : A_i=0\}} Y_i - \min_{\{i : A_i=0\}} Y_i\right) \left(\frac{1}{2} - \frac{1}{n-2}\right), \quad (\text{B.1})$$

and

$$E\left(\hat{\Delta}_{blind}(\mathbf{X}, \mathbf{Y})\right) - \Delta \leq E_{\mathbf{X}} \left\{ \max_{\{i : A_i=0\}} \mu(\mathbf{X}_i, A_i) - \min_{\{i : A_i=0\}} \mu(\mathbf{X}_i, A_i) \right\} \left(\frac{1}{2} - \frac{1}{n-2}\right). \quad (\text{B.2})$$

The upper bounds in Eqs B.1 & B.2 are tight in the sense that, if  $(\mathbf{X}_1, \dots, \mathbf{X}_p)$  contains an arbitrarily large number independent Bernoulli variables, then the difference between the left and right-hand sides slowly approaches zero as  $p \rightarrow \infty$ , with  $n$  held fixed. Alternatively, if analysts can adaptively define any categorical feature they wish to adjust for, then both Eq (B.1) & Eq (B.2) hold with equality.

Roughly speaking, the right-hand side of Eq (B.1) represents the potential bias incurred by isolating the extremes of a particular sample. Thus, if  $\tilde{Y}^{control}$  is a continuous variable with nonnegative support across the real line, then the worst-case bias of  $\hat{\Delta}_{snoop}$  slowly diverges towards infinity as the sample size grows. For example, if  $\tilde{Y}^{control}$  follows a standard normal distribution, then the worst-case bias grows at a rate approximately proportional to  $\sqrt{\log(n/2)}$  (see Theorem 1.5.3 of Leadbetter et al., 1983).

Similarly, the right-hand side of Eq (B.2) represents the bias incurred by upweighting datapoints that are *expected* to be extreme, with more informative features  $\mathbf{X}$  leading to higher bias. Continuing the above example, if  $\tilde{Y}^{control}$  and  $E(Y_i | \mathbf{X}, A_i = 0)$  follow a joint normal distribution, then the right-hand side of Eq (B.2) also diverges towards infinity, and is proportional to the right-hand side of Eq (B.1) (see Figure B.2 for an illustration). This proportional relationship is consistent with our discussion in Section 2.2.

A crucial caveat however is that the upper bounds in Theorem B.1 are only achieved when analysts are able to justify adjustment on arbitrarily complex variables, or when  $p$  is dramatically larger than  $n$ .

## C Additional simulation results

Figures C.1 & C.2 show the simulation results for  $d_{IPW}$ , which are extremely similar to the results for  $d_{OLS}$  (see Figures 2 & 3).

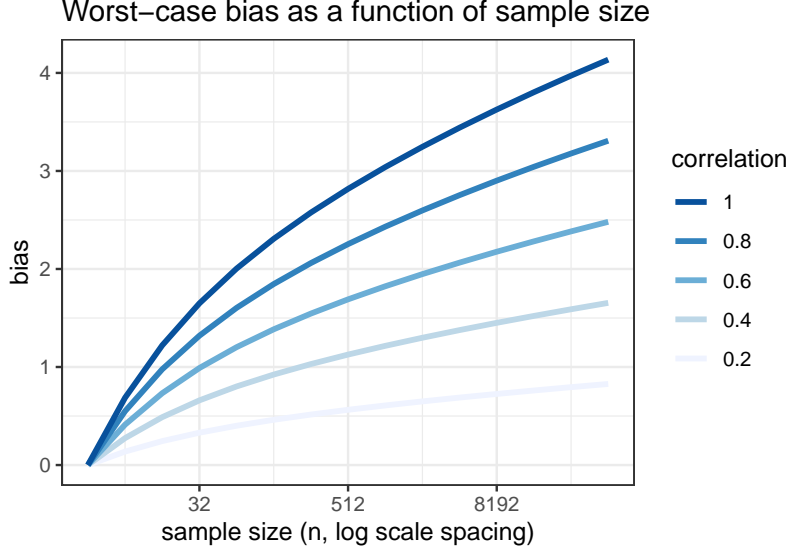

Figure B.2: Worst-case bias in the blinded setting – Above, we illustrate the multivariate normal setting described in Section B. Here, the worst-case bias is a function of the sample size and the correlation between  $\mu(\mathbf{X}_i, 0)$  and  $Y_i$ , given  $A_i = 0$ . When this correlation is 1, we recover the worst-case bias from the unblinded setting. Otherwise, the worst-case bias in the blinded setting grows proportionally to the worst-case bias in the unblinded setting. It is important to note that in order for this worst-case bias to be achieved,  $p$  must grow much faster than  $n$ .

## D Helpful relationships used in proofs

In the proofs that follow, we will make references to several helpful properties of  $d(\mathbf{X}_j, \mathbf{Y})$ . These properties hold whenever the estimator function  $d$  is either  $d_{\text{OLS}}$  or  $d_{\text{IPW}}$ .

The first property is linearity with respect to  $\mathbf{Y}$ , which we require by the definition of  $d$ . This means that  $d(\mathbf{X}_j, c\mathbf{Y} + \mathbf{Z}) = cd(\mathbf{X}_j, \mathbf{Y}) + d(\mathbf{X}_j, \mathbf{Z})$  for any random variable  $\mathbf{Z}$  and constant  $c$ . Linearity also implies that

$$d(\mathbf{X}_j, \mathbf{Y} + c\mathbf{1}) = d(\mathbf{X}_j, \mathbf{Y}) \quad (\text{D.1})$$

for any constant  $c$ , as  $d(\mathbf{X}_j, \mathbf{1}c) = 0$ .

Next, for binary treatments  $\mathbf{A} \in \{0, 1\}^n$ , we note that  $d(\mathbf{X}_j, \mathbf{A}) = 1$ . Combining, this with linearity implies that

$$d(\mathbf{X}_j, \mathbf{Y} + c\mathbf{A}) = d(\mathbf{X}_j, \mathbf{Y}) + c. \quad (\text{D.2})$$

Finally, we note that  $d(\mathbf{X}_j, \mathbf{Y})$  is invariant to the scale of  $\mathbf{X}_j$ . That is,

$$d(c\mathbf{X}_j, \mathbf{Y}) = d(\mathbf{X}_j, \mathbf{Y}) \quad (\text{D.3})$$

for any nonzero constant  $c$ .

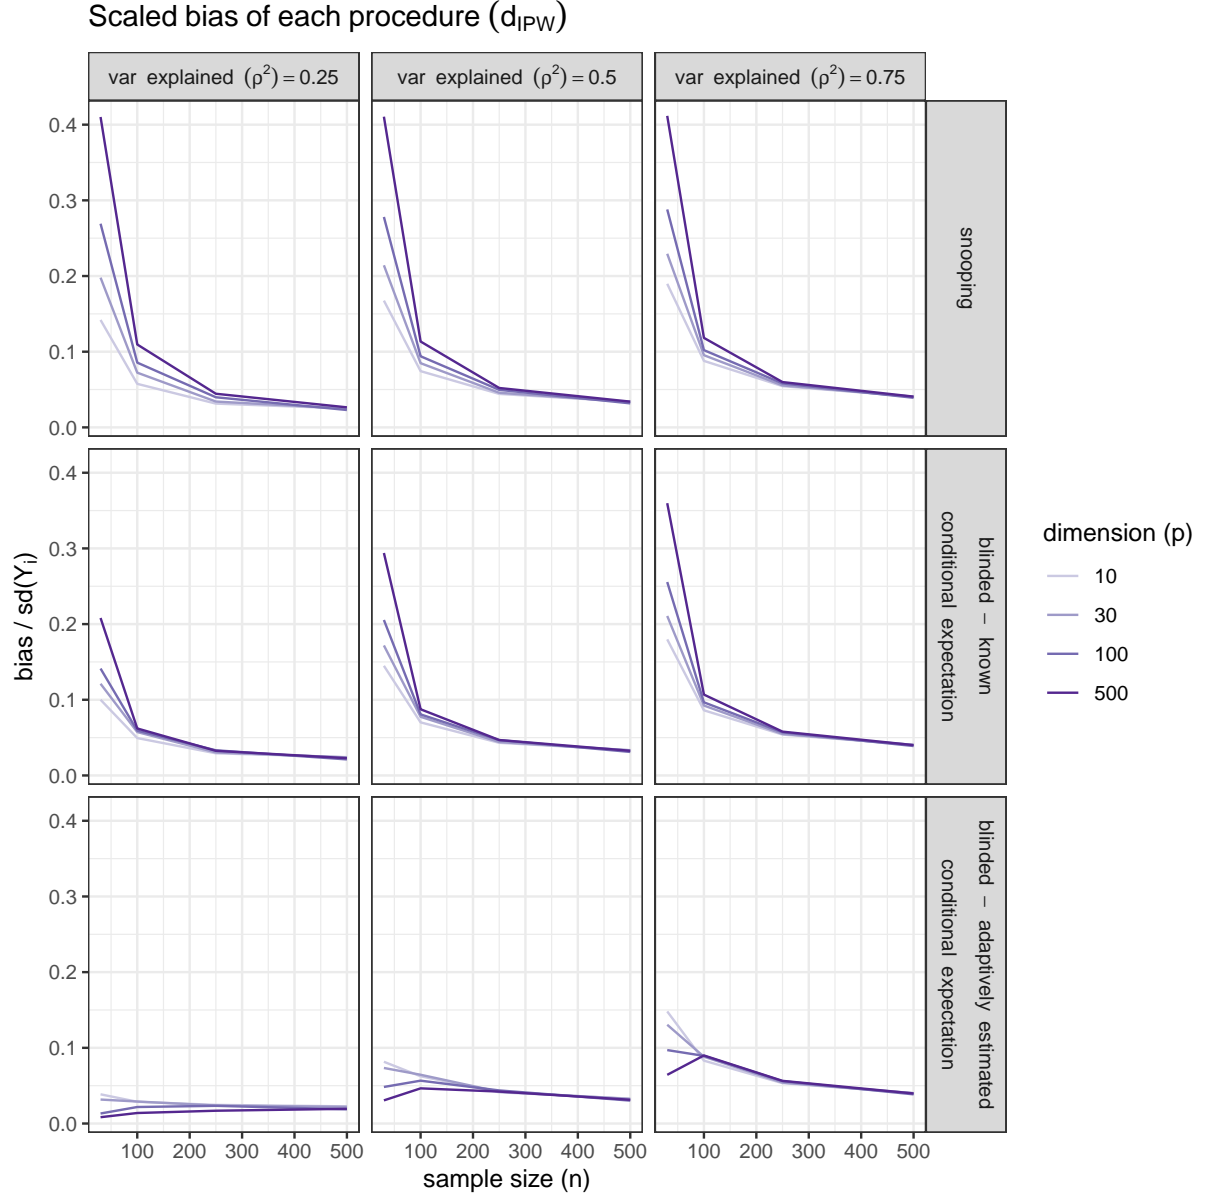

Figure C.1: Simulated bias from snooping and blinded analysts using  $d_{IPW}$  – Results above are organized in the same way as in Figure 2.

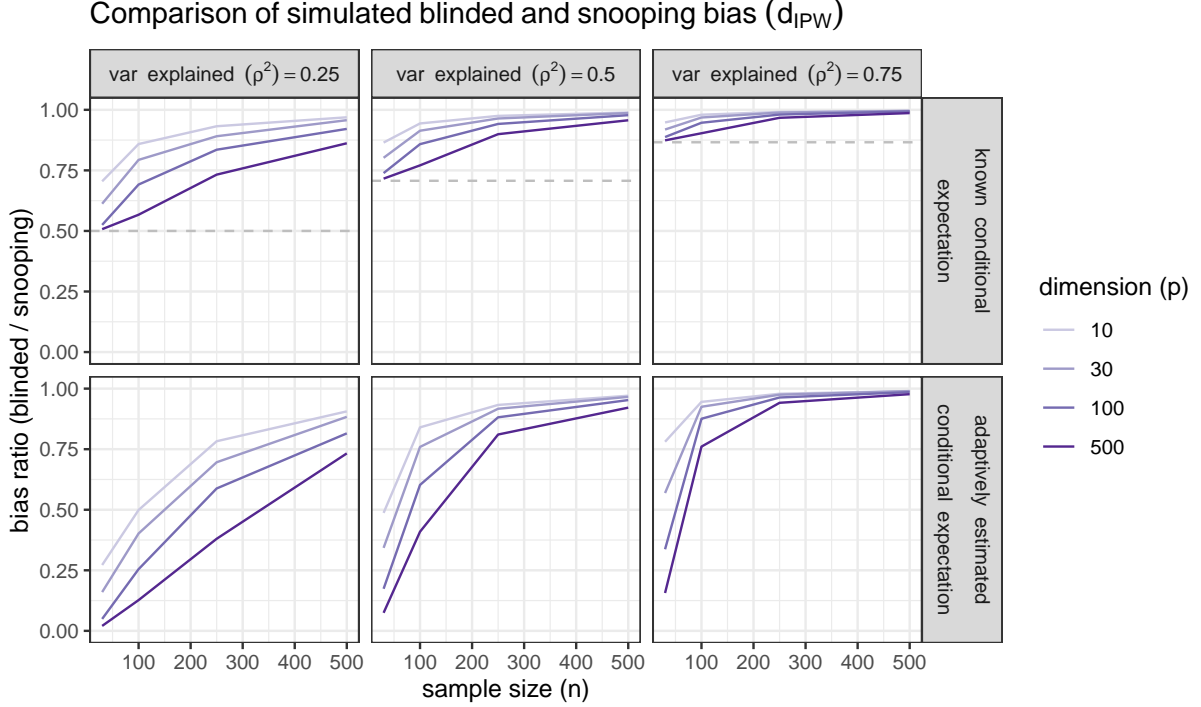

Figure C.2: Comparison of bias from simulated snooping and blinded analysts, each using  $d_{IPW}$  – Results above are organized in the same way as in Figure 3.

## E Proof of Theorem 1 and its corollaries

### E.1 Proof of Theorem 1

To help motivate the steps of our proof, we first sketch our overall approach. We will start by expressing each analysts’ ranks using results from linear mediation (or, equivalently, the “omitted variable formula”). We’ll note that the adjusted estimator  $d(\mathbf{X}_j, \mathbf{Y})$  can be written as the “direct effect” of  $A$ , which is equal to the “total effect” of  $A$  minus the “indirect effect” of  $A$ . The total effect is constant across features, so it does not affect the rankings. For the snooping analyst, the indirect effect depends on  $\mathbf{A}^\top \mathbf{X}$  and  $\mathbf{Y}^\top \mathbf{X}$ . Similarly, for the blinded analyst, the indirect effect depends on  $\mathbf{A}^\top \mathbf{X}$  and  $\mu(\mathbf{X}, \mathbf{A})^\top \mathbf{X}$ . In large samples,  $\frac{1}{n} \mu(\mathbf{X}, \mathbf{A})^\top \mathbf{X}$  approximates  $\frac{1}{n} \mathbf{Y}^\top \mathbf{X}$ , and so two analysts make their rankings from similar information. Finally, we’ll see that, for this reason, the rankings of the blinded and snooping analyst converge to each other.

#### E.1.1 Preliminaries: mediation and omitted variables in linear regression

This subsection introduces several preliminaries before we proceed with the main part of the proof. We will assume WLOG that

$$|Cor(X_{j,i}, X_{k,i})| < 1; \quad Cor(X_{j,i}, \mu(\mathbf{X}_i, A_i)), Cor(X_{k,i}, \mu(\mathbf{X}_i, A_i)) > 0; \quad (\text{E.1})$$

and

$$Var(X_{j,i}) = Var(X_{k,i}) = 1. \quad (\text{E.2})$$

The first simplification is possible WLOG because if  $Cor(X_{j,i}, X_{k,i}) = 1$ , then the strict inequalities in Eq (4) cause the left-hand side of Eq (4) to be zero, regardless of  $n$ . The second two simplifications are possible WLOG because multiplying  $\mathbf{X}_j$  by -1 does not change either the estimate  $d(\mathbf{X}_j, \mathbf{Y})$  or the rankings of either analyst (see Eq (D.3)). The same is true of scaling  $\mathbf{X}_j$  by a nonzero constant. So, in cases where  $Cor(X_{j,i}, \mu(\mathbf{X}_i, A_i)) < 0$  or  $Var(X_{j,i}) \neq 1$ , we can simply rescale  $\mathbf{X}_j$  appropriately without substantively changing the problem.

First, we consider rankings of the “snooping” analyst. By assumption, the estimate  $d(\mathbf{x}_j, \mathbf{y}) = d_{OLS}(\mathbf{x}_j, \mathbf{y})$  comes from fitting a linear regression model. Let,

$$\left( \hat{\beta}_0, \hat{\beta}_j, d(\mathbf{x}_j, \mathbf{y}) \right) = \arg \min_{b_0, b_j, b_a} \| \mathbf{y} - (b_0 + b_j \mathbf{x}_j + b_a \mathbf{a}) \|^2_2. \quad (\text{E.3})$$

Above, we suppress the dependence of  $\hat{\beta}_0$  on  $j$  for simplicity, as  $\hat{\beta}_0$  will not play an important role in the proof.

Standard results for omitted variables (e.g., Section 9.2.1 of Seber and Lee, 2003) show that

$$d(\mathbf{x}_j, \mathbf{y}) = \hat{\Delta}_0 - \hat{\beta}_j \hat{\gamma}_j, \quad (\text{E.4})$$

where  $\hat{\gamma}_j$  is the best fitting coefficient defined from

$$(\hat{\gamma}_0, \hat{\gamma}_j) = \arg \min_{c_0, c_j} \| \mathbf{x}_j - (c_0 + c_j \mathbf{a}) \|^2_2, \quad (\text{E.5})$$

and  $\hat{\Delta}_0$  is the unadjusted difference in sample means:

$$\frac{1}{n/2} \left( \sum_{i=1+n/2}^n y_i \right) - \frac{1}{n/2} \left( \sum_{i=1}^{n/2} y_i \right). \quad (\text{E.6})$$

Again, for simplicity, we suppress the dependence of  $\hat{\gamma}_0$  on  $j$ .

In words, Eq (E.4) is often summarized by saying that the “total effect” ( $\hat{\Delta}_0$ ) is the sum of the “direct effect” ( $d(\mathbf{x}_j, \mathbf{y})$ ) and the “indirect effect” ( $\hat{\beta}_j \hat{\gamma}_j$ ). Thus, if  $R_{j, \text{snoop}} > R_{k, \text{snoop}}$ , it must be that

$$\begin{aligned} d(\mathbf{X}_j, \mathbf{Y}) &< d(\mathbf{X}_k, \mathbf{Y}) \\ \hat{\Delta}_0 - \hat{\beta}_j \hat{\gamma}_j &< \hat{\Delta}_0 - \hat{\beta}_k \hat{\gamma}_k \\ \hat{\beta}_k \hat{\gamma}_k &< \hat{\beta}_j \hat{\gamma}_j. \end{aligned} \quad (\text{E.7})$$

Similarly, the blinded analyst ranks features by fitting linear models with  $\mu(\mathbf{X}, \mathbf{A})$  as the outcome. Let,

$$\left( \tilde{\beta}_0, \tilde{\beta}_j, d(\mathbf{x}_j, \mu(\mathbf{x}, \mathbf{a})) \right) = \arg \min_{b_0, b_j, b_a} \| \mu(\mathbf{x}, \mathbf{a}) - (b_0 + b_j \mathbf{x}_j + b_a \mathbf{a}) \|^2_2,$$

where  $d(\mathbf{x}_j, \mu(\mathbf{x}, \mathbf{a}))$  is the blinded analyst’s best guess of the unblinded estimate  $d(\mathbf{x}_j, \mathbf{y})$ . As before,

$$d(\mathbf{x}_j, \mu(\mathbf{x}, \mathbf{a})) = \tilde{\Delta}_0 - \tilde{\beta}_j \hat{\gamma}_j,$$

where  $\tilde{\Delta}_0$  can be computed by replacing  $y_i$  with  $\mu(\mathbf{x}_i, a_i)$  in Eq (E.6), and  $\hat{\gamma}_j$  is again the best fitting OLS coefficient from Eq (E.5). Thus, if  $R_{j,\text{blind}} < R_{k,\text{blind}}$ , it must be that

$$\begin{aligned} d(\mathbf{x}_j, \mu(\mathbf{x}, \mathbf{a})) &> d(x_k, \mu(\mathbf{x}, \mathbf{a})) \\ \tilde{\beta}_k \hat{\gamma}_k &> \tilde{\beta}_j \hat{\gamma}_j. \end{aligned} \tag{E.8}$$

Comparing the ranking information in Eqs E.7 & E.8, two similarities become apparent. First, we see that value of  $(\hat{\gamma}_j, \hat{\gamma}_k)$  is visible to both analysts, and appears in both Eq (E.7) & Eq (E.8). Second, while  $(\hat{\beta}_j, \hat{\beta}_k)$  does not equal  $(\tilde{\beta}_j, \tilde{\beta}_k)$ , the law of large numbers and Slutsky's Theorem imply that these statistics converge in probability to the same constants. From Condition 3 we have

$$\begin{aligned} \hat{\beta}_j &\rightarrow_p \text{Var}(X_{j,i})^{-1} \text{Cov}(X_{j,i}, Y_i) \\ &= \text{Var}(X_{j,i})^{-1} \text{Cov}(X_{j,i}, Y_i - \mu(\mathbf{X}_i, A_i) + \mu(\mathbf{X}_i, A_i)) \\ &= \text{Var}(X_{j,i})^{-1} \{ \text{Cov}(X_{j,i}, Y_i - \mu(\mathbf{X}_i, A_i)) + \text{Cov}(X_{j,i}, \mu(\mathbf{X}_i, A_i)) \} \\ &= \text{Var}(X_{j,i})^{-1} \text{Cov}(X_{j,i}, \mu(\mathbf{X}_i, A_i)), \end{aligned} \tag{E.9}$$

and

$$\tilde{\beta}_j \rightarrow_p \text{Var}(X_{j,i})^{-1} \text{Cov}(X_{j,i}, \mu(\mathbf{X}_i, A_i)).$$

Let  $\beta_j$  denote this common limit, which must be strictly positive because of our simplifying assumption that  $0 < \text{Cor}(\mathbf{X}_j, \mu(\mathbf{X}, \mathbf{A}))$  (see Eq (E.1)).

As a result,  $(\hat{\beta}_j/\hat{\beta}_k)$  and  $(\tilde{\beta}_j/\tilde{\beta}_k)$  both converge in probability to  $\beta_j/\beta_k > 0$ . In more explicit notation, this means that for any arbitrarily small constants  $h, \delta \in (0, 1]$  and there exists a constant  $n_{h,\delta}$  such that, for all  $n \geq n_{h,\delta}$ , the following three conditions hold:

$$P \left( \left| \frac{\hat{\beta}_j}{\hat{\beta}_k} - \frac{\beta_j}{\beta_k} \right| > \delta \right) < h, \tag{E.10}$$

$$P \left( \left| \frac{\tilde{\beta}_j}{\tilde{\beta}_k} - \frac{\beta_j}{\beta_k} \right| > \delta \right) < h, \tag{E.11}$$

and

$$P \left( \min \{ \tilde{\beta}_k, \hat{\beta}_k, \tilde{\beta}_j, \hat{\beta}_j \} < 0 \right) < h. \tag{E.12}$$

In contrast, the distribution of  $\hat{\gamma}_j/\hat{\gamma}_k$  does *not* approach a constant. To see this, note that because  $\mathbf{A}$  is fixed,  $\hat{\gamma}_j$  and  $\hat{\gamma}_k$  are equivalent to differences in means for  $\mathbf{X}_j$  and  $\mathbf{X}_k$  across the two treatment arms. From the multivariate central limit theorem,  $\hat{\gamma}_j$  and  $\hat{\gamma}_k$  converge to a multivariate normal distribution centered at zero (see Condition 3), and so their ratio does not converge to a constant. Specifically,

$$\sqrt{\frac{n}{2}} \begin{pmatrix} \hat{\gamma}_j \\ \hat{\gamma}_k \end{pmatrix} \rightarrow_d N \left( \begin{pmatrix} 0 \\ 0 \end{pmatrix}, \Sigma_{jk} \right), \tag{E.13}$$

where

$$\Sigma_{jk} = \begin{bmatrix} 2 & \sigma_{jk}^2 \\ \sigma_{jk}^2 & 2 \end{bmatrix},$$

and

$$\begin{aligned} \sigma_{jk}^2 &= \text{Cov}(X_{j,i+n/2} - X_{j,i}, X_{k,i+n/2} - X_{k,i}) && \text{for any } i \in \{1, \dots, n/2\} \\ &= 2\text{Cov}(X_{j,i}, X_{k,i}) \\ &< 2 && \text{from Eq (E.2).} \end{aligned}$$

We're now equipped to prove Theorem 1.

### E.1.2 Showing Eq (4)

*Proof.* In this section, we will use the notation and preliminaries from Section E.1.1 to prove Theorem 1. We will show that when  $\hat{\gamma}_j\beta_j < \hat{\gamma}_k\beta_k$  it is unlikely for either analyst to rank  $\mathbf{X}_k$  before  $\mathbf{X}_j$ , and when  $\hat{\gamma}_j\beta_j \geq \hat{\gamma}_k\beta_k$  it is unlikely for either analyst to rank  $\mathbf{X}_j$  before  $\mathbf{X}_k$ . That is, the blinded and snooping analysts' rankings both typically agree with the order of  $\hat{\gamma}_1\beta_1, \dots, \hat{\gamma}_p\beta_p$ . As a result, the rankings from the two analysts will also tend to agree with each other.

For any  $h, \delta$ , let  $n_{h,\delta}$  be defined as above. Hereafter, we will assume that  $n \geq n_{h,\delta}$ .

The left-hand side of Eq (4) can be broken up into two parts:

$$P(R_{j,\text{blind}} < R_{k,\text{blind}}; R_{j,\text{snoop}} > R_{k,\text{snoop}}) \tag{E.14}$$

$$= P(R_{j,\text{blind}} < R_{k,\text{blind}}; R_{j,\text{snoop}} > R_{k,\text{snoop}}; \hat{\gamma}_j\beta_j < \hat{\gamma}_k\beta_k) \tag{E.15}$$

$$+ P(R_{j,\text{blind}} < R_{k,\text{blind}}; R_{j,\text{snoop}} > R_{k,\text{snoop}}; \hat{\gamma}_j\beta_j \geq \hat{\gamma}_k\beta_k). \tag{E.16}$$

We'll start by upper bounding Line E.15. Writing this line in terms of  $\hat{\beta}_j, \hat{\gamma}_j, \hat{\beta}_k$ , and  $\hat{\gamma}_k$  gives

$$\begin{aligned} &P(R_{j,\text{blind}} < R_{k,\text{blind}}; R_{j,\text{snoop}} > R_{k,\text{snoop}}; \hat{\gamma}_j\beta_j < \hat{\gamma}_k\beta_k) \\ &\leq P(R_{j,\text{snoop}} > R_{k,\text{snoop}}; \hat{\gamma}_j\beta_j < \hat{\gamma}_k\beta_k) \\ &= P(\hat{\beta}_j\hat{\gamma}_j > \hat{\beta}_k\hat{\gamma}_k; \hat{\gamma}_j\beta_j < \hat{\gamma}_k\beta_k) && \text{from Eq (E.7)} \\ &\leq P(\hat{\beta}_j\hat{\gamma}_j > \hat{\beta}_k\hat{\gamma}_k; \hat{\gamma}_j\beta_j < \hat{\gamma}_k\beta_k; 0 < \hat{\beta}_j, \hat{\beta}_k) + h && \text{from Eq (E.12)} \\ &= P\left(\frac{\hat{\beta}_j}{\hat{\beta}_k}\hat{\gamma}_j > \hat{\gamma}_k; \frac{\beta_j}{\beta_k}\hat{\gamma}_j < \hat{\gamma}_k; 0 < \hat{\beta}_j, \hat{\beta}_k\right) + h. \\ &\leq P\left(\frac{\beta_j}{\beta_k}\hat{\gamma}_j < \hat{\gamma}_k < \frac{\hat{\beta}_j}{\hat{\beta}_k}\hat{\gamma}_j; 0 < \frac{\hat{\beta}_j}{\hat{\beta}_k}\right) + h. \end{aligned} \tag{E.17}$$

For ease of notation, let  $w = \beta_j/\beta_k > 0$  and let  $\hat{W} = \hat{\beta}_j/\hat{\beta}_k$ . Plugging this into Line E.17

give

$$\begin{aligned}
& P(R_{j,\text{blind}} < R_{k,\text{blind}}; R_{j,\text{snoop}} > R_{k,\text{snoop}}; \hat{\gamma}_j \beta_j < \hat{\gamma}_k \beta_k) \\
& \leq P\left(w\hat{\gamma}_j < \hat{\gamma}_k < \hat{W}\hat{\gamma}_j; 0 < \hat{W}\right) + h. \\
& = P\left(w\hat{\gamma}_j < \hat{\gamma}_k < \hat{W}\hat{\gamma}_j; 0 < \hat{W}; \text{sign}(\hat{\gamma}_j) = \text{sign}(\hat{\gamma}_k)\right) + h
\end{aligned} \tag{E.18}$$

$$= P\left(0 < w\hat{\gamma}_j < \hat{\gamma}_k < \hat{W}\hat{\gamma}_j; 0 < \hat{W}\right) \tag{E.19}$$

$$+ P\left(w\hat{\gamma}_j < \hat{\gamma}_k < \hat{W}\hat{\gamma}_j < 0; 0 < \hat{W}\right) + h \tag{E.20}$$

$$\leq P(w\hat{\gamma}_j < \hat{\gamma}_k < (w + \delta)\hat{\gamma}_j) \tag{E.21}$$

$$+ P(w\hat{\gamma}_j < \hat{\gamma}_k < (w - \delta)\hat{\gamma}_j) + 3h. \tag{E.22}$$

Above, in Line E.18, we use that fact that since  $0 < w, \hat{W}$ , we know that if  $\hat{\gamma}_j > 0$  then  $\hat{\gamma}_k$  is in-between two positive numbers. Likewise, if  $\hat{\gamma}_j < 0$ , then  $\hat{\gamma}_k$  is in-between two negative numbers. In Lines (E.19) & (E.20), we consider these two cases separately ( $\hat{\gamma}_j, \hat{\gamma}_k < 0$  versus  $0 < \hat{\gamma}_j, \hat{\gamma}_k$ ), which then lets us apply Eq (E.10) in Lines (E.21) & (E.22).

Let  $B_{\delta,+}$  and  $B_{\delta,-}$  be the linear cones satisfying the inequalities in Lines (E.21) & (E.22) respectively. That is, let

$$\begin{aligned}
B_{\delta,+} &= \{(z_1, z_2) \in \mathbb{R}^2 : wz_1 < z_2 < (w + \delta)z_1\}, \text{ and} \\
B_{\delta,-} &= \{(z_1, z_2) \in \mathbb{R}^2 : wz_1 < z_2 < (w - \delta)z_2\}.
\end{aligned}$$

Plugging this into Lines (E.21) & (E.22) gives

$$\begin{aligned}
& P(R_{j,\text{blind}} < R_{k,\text{blind}}; R_{j,\text{snoop}} > R_{k,\text{snoop}}; \hat{\gamma}_j \beta_j < \hat{\gamma}_k \beta_k) \\
& \leq P((\hat{\gamma}_j, \hat{\gamma}_k) \in B_{\delta,+}) + P((\hat{\gamma}_j, \hat{\gamma}_k) \in B_{\delta,-}) + 3h. \\
& = P\left(\sqrt{\frac{n}{2}}(\hat{\gamma}_j, \hat{\gamma}_k) \in B_{\delta,+}\right) + P\left(\sqrt{\frac{n}{2}}(\hat{\gamma}_j, \hat{\gamma}_k) \in B_{\delta,-}\right) + 3h. \\
& \rightarrow P((Z_1, Z_2) \in B_{\delta,+}) + P((Z_1, Z_2) \in B_{\delta,-}) + 3h. \quad \text{from Eq (E.13), (E.24)}
\end{aligned} \tag{E.23}$$

where  $(Z_1, Z_2)$  is a random vector with distribution  $N(\mathbf{0}, \Sigma_{jk})$ . Since  $\text{Cor}(Z_1, Z_2) < 1$ , the probabilities  $P((Z_1, Z_2) \in B_{r,\delta,+})$  and  $P((Z_1, Z_2) \in B_{r,\delta,-})$  can be made arbitrarily small by decreasing  $\delta$ , regardless of the value of  $\sigma_{jk}^2 < 2$  (see illustration in Figure E.1, as well as Section E.1.3 for details). Thus, Line (E.23) converges to an arbitrarily small quantity.

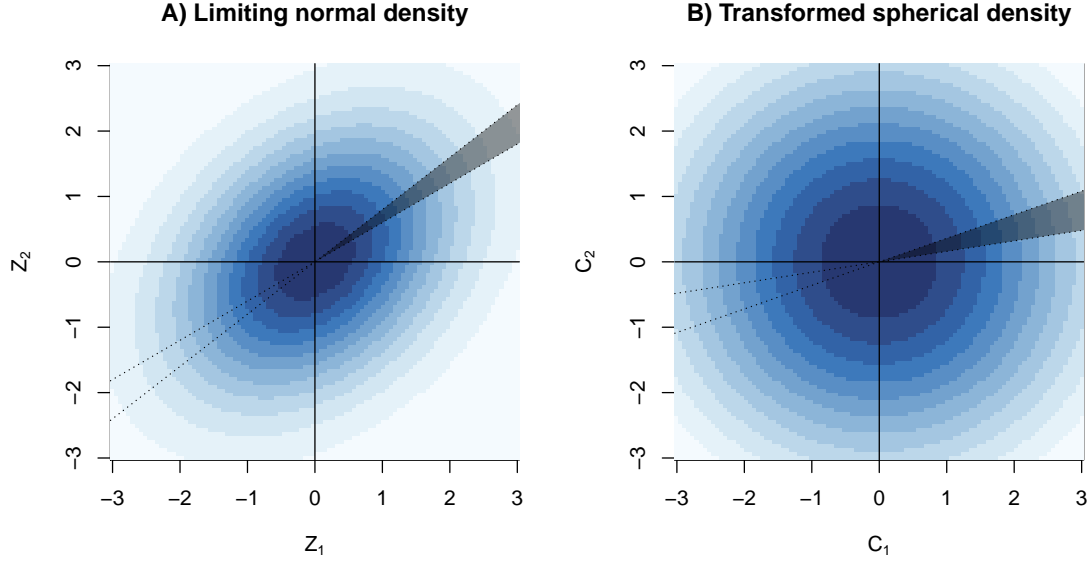

Figure E.1: Limiting density for  $(Z_1, Z_2)$ : **Panel A** shows a hypothetical region  $B_{\delta,+}$  for  $\delta = 0.2$  and  $w = 0.6$  in gray. The linear constraints of this region are represented by dotted lines with slopes of  $(w + \delta)$  and  $w$ . The interior of the region is marked by shading. We overlay the density of bivariate normal with variance  $\Sigma_{jk}$ , and  $\sigma_{jk}^2 = 0.7$ . We can see that reducing  $\delta$  can make the probability of the shaded region arbitrarily small. A more formal proof of this fact can be seen by changing the coordinate system such that  $(Z_1, Z_2)$  that follows a spherical distribution, as in **Panel B**. The transformed shaded region then has probability equal to the proportion of the unit circle that it covers. Again, this proportion can be made arbitrarily small by decreasing  $\delta$  (see details in Section E.1.3).

We can follow the same steps for Line (E.16). Let  $\tilde{W} = \tilde{\beta}_j / \tilde{\beta}_k$ . Then

$$\begin{aligned}
& P(R_{j,\text{blind}} < R_{k,\text{blind}}; R_{j,\text{snoop}} > R_{k,\text{snoop}}; \hat{\gamma}_j \beta_j \geq \hat{\gamma}_k \beta_k) \\
& \leq P(R_{j,\text{blind}} < R_{k,\text{blind}}; \hat{\gamma}_j \beta_j \geq \hat{\gamma}_k \beta_k) \\
& = P\left(\hat{\gamma}_j \tilde{\beta}_j < \hat{\gamma}_k \tilde{\beta}_k; \quad \hat{\gamma}_j \beta_j \geq \hat{\gamma}_k \beta_k\right) \\
& \leq P\left(\hat{\gamma}_j \tilde{\beta}_j < \hat{\gamma}_k \tilde{\beta}_k; \quad \hat{\gamma}_j \beta_j \geq \hat{\gamma}_k \beta_k; \quad 0 < \tilde{\beta}_j, \tilde{\beta}_k\right) + h \\
& = P\left(\hat{\gamma}_j \frac{\tilde{\beta}_j}{\tilde{\beta}_k} < \hat{\gamma}_k; \quad \hat{\gamma}_j \frac{\beta_j}{\beta_k} \geq \hat{\gamma}_k; \quad 0 < \tilde{\beta}_j, \tilde{\beta}_k\right) + h \\
& \leq P\left(\hat{\gamma}_j \tilde{W} < \hat{\gamma}_k \leq \hat{\gamma}_j w; \quad 0 < \tilde{W}\right) + h \\
& = P\left(\hat{\gamma}_j \tilde{W} < \hat{\gamma}_k \leq \hat{\gamma}_j w \leq 0; \quad 0 < \tilde{W}\right) \\
& \quad + P\left(0 < \hat{\gamma}_j \tilde{W} < \hat{\gamma}_k \leq \hat{\gamma}_j w; \quad 0 < \tilde{W}\right) + h \\
& \leq P(\hat{\gamma}_j(w + \delta) < \hat{\gamma}_k \leq \hat{\gamma}_j w) \\
& \quad + P(\hat{\gamma}_j(w - \delta) < \hat{\gamma}_k \leq \hat{\gamma}_j w) + 3h. \\
& \rightarrow P(Z_1(w + \delta) < Z_2 \leq Z_1 w) \tag{E.25} \\
& \quad + P(Z_1(w - \delta) < Z_2 \leq Z_1 w) + 3h. \tag{E.26}
\end{aligned}$$

where  $(Z_1, Z_2)$  is a random vector with distribution  $N(\mathbf{0}, \Sigma_{jk})$ . Again, the two probabilities in Lines (E.25)-(E.26) can be made arbitrarily small by decreasing  $\delta$ . Together with Eq (E.24), we see that the probability in Line (E.14) converges to a quantity that can be made arbitrarily small by decreasing  $\delta$  and  $h$ .  $\square$

### E.1.3 Supplemental details on spherical distributions

In this section we show that the probabilities in Lines E.24, E.25 & E.26 can be made arbitrarily small by decreasing  $\delta$ .

Let  $(Z_1, Z_2)$  be a random vector with distribution  $N(\mathbf{0}, \Sigma_{jk})$ , as defined in the previous section. Let  $C_1 = Z_1 + Z_2$  and let  $C_2 = v(Z_1 - Z_2)$  with  $v = \sqrt{\frac{2 + \sigma_{jk}^2}{2 - \sigma_{jk}^2}}$ . Then, using Eq (E.1),

$$\begin{aligned}
Cov(C_1, C_2) &= v \{Cov(Z_1 + Z_2, Z_1 - Z_2)\} \\
&= v \{Cov(Z_1, Z_1) - Cov(Z_1, Z_2) + Cov(Z_2, Z_1) - Cov(Z_2, Z_2)\} \\
&= v \{Cov(Z_1, Z_1) - Cov(Z_2, Z_2)\} \\
&= 0.
\end{aligned}$$

We see that

$$\begin{aligned}
Var(C_2) &= v^2 (Var(Z_1) + Var(Z_2) - 2\sigma_{jk}^2) \\
&= v^2 (4 - 2\sigma_{jk}^2) \\
&= 4 + 2\sigma_{jk}^2 \\
&= Var(C_1).
\end{aligned}$$

Since  $(C_1, C_2)$  is a linear combination of a multivariate normal, it also follows a multivariate normal distribution.

In particular, the above relations show that  $(C_1, C_2)$  follows a *spherical* normal distribution. As a result, it is simple to evaluate the probability that  $(C_1, C_2)$  falls in cone regions of the form  $\mathcal{C} = \{(c_1, c_2) : c_1 l < c_2 < c_1 u\}$ , for arbitrary constants  $l, u \in \mathbb{R}$  (see example in Figure E.1-B). Specifically,  $(C_1, C_2) \in \mathcal{C}$  indicates that the point  $(C_1, C_2)$  is above the line through the origin with slope  $l$ , and below the line through the origin with slope  $u$ . The probability of this event depends on the angle between the vectors  $(1, u)$  and  $(1, l)$ , which have slopes  $l$  and  $u$  respectively. That is,

$$P((C_1, C_2) \in \mathcal{C}) = \frac{1}{2\pi} \cos^{-1} \left( \frac{1 + ul}{\sqrt{1 + u^2} \sqrt{1 + l^2}} \right), \quad (\text{E.27})$$

where the inverse cosine term is the angle between  $(1, u)$  and  $(1, l)$ .

Being able to describe the distribution of  $(C_1, C_2)$ , we now need to translate statements about  $(Z_1, Z_2)$  into equivalent statements about  $(C_1, C_2)$ . To do this, note that

$$Z_1 = \frac{1}{2} \left( C_1 + \frac{C_2}{v} \right), \text{ and } Z_2 = \frac{1}{2} \left( C_1 - \frac{C_2}{v} \right).$$

Now, for any two constants  $a, b > 0$ , we have

$$\begin{aligned} & P(aZ_1 < Z_2 < bZ_1) \\ &= P(a(C_1 + C_2 v^{-1}) < C_1 - C_2 v^{-1} < b(C_1 + C_2 v^{-1})) \\ &= P(a(vC_1 + C_2) < vC_1 - C_2 < b(vC_1 + C_2)) \\ &= P(a(vC_1 + C_2) < vC_1 - C_2; \\ &\quad vC_1 - C_2 < b(vC_1 + C_2)) \\ &= P(C_2(1 + a) < vC_1(1 - a); \\ &\quad vC_1(1 - b) < C_2(1 + b)) \\ &= P\left(C_2 < vC_1 \frac{1 - a}{1 + a}; \right. \\ &\quad \left. vC_1 \frac{1 - b}{1 + b} < C_2\right) \\ &= P\left(C_1 v \frac{1 - b}{1 + b} < C_2 < C_1 v \frac{1 - a}{1 + a}\right) \\ &= \frac{1}{2\pi} \cos^{-1} \left( \frac{1 + v^2 \left(\frac{1-a}{1+a}\right) \left(\frac{1-b}{1+b}\right)}{\sqrt{1 + v^2 \left(\frac{1-a}{1+a}\right)^2} \sqrt{1 + v^2 \left(\frac{1-b}{1+b}\right)^2}} \right) \quad \text{from Eq (E.27)} \quad (\text{E.28}) \end{aligned}$$

This quantity can be made arbitrarily small by moving  $a$  and  $b$  closer together.

Finally, we can plug either  $(w - \delta, w)$ ;  $(w + \delta, w)$ ;  $(w, w - \delta)$ ; or  $(w, w + \delta)$  in for  $(a, b)$  in Eq (E.28) to see that  $P((w - \delta)Z_1 < Z_2 < wZ_1)$ ;  $P((w + \delta)Z_1 < Z_2 < wZ_1)$ ;  $P(wZ_1 < Z_2 < (w - \delta)Z_1)$ ; and  $P(wZ_1 < Z_2 < (w + \delta)Z_1)$  all can be made arbitrarily small by decreasing  $\delta$ .

## E.2 Proof of Corollary 6

The proof of Corollary 6 will be almost identical to that of the proof for Theorem 1. In the proof of Theorem 1, the only place where we used that fact that  $\mu(\mathbf{X}, \mathbf{A}) = E(\mathbf{Y}|\mathbf{X}, \mathbf{A})$  was in showing that  $\hat{\beta}_j$  and  $\tilde{\beta}_j$  converge to a common limit. Thus, all that remains is to show that  $\hat{\beta}_j$  and  $\tilde{\beta}_j$  still converge to a common limit as  $n, n_{\text{train}} \rightarrow \infty$  if we replace  $\mu(\mathbf{X}, \mathbf{A})$  with  $\mu_{n_{\text{train}}}(\mathbf{X}, \mathbf{A})$  and add the assumption that  $E[(\mu_{n_{\text{train}}}(\mathbf{X}_i, A_i) - \mu(\mathbf{X}_i, A_i))^2] \rightarrow 0$  as  $n_{\text{train}} \rightarrow \infty$ . The definition of  $\hat{\beta}_j$  is unchanged.

Since  $E[(\mu_{n_{\text{train}}}(\mathbf{X}_i, A_i) - \mu(\mathbf{X}_i, A_i))^2] \rightarrow 0$ , there must exist a value  $k$  such that  $\text{Var}(\mu_{n_{\text{train}}}(\mathbf{X}_i, A_i))$  is bounded for any  $n_{\text{train}} > k$ . For any such  $n_{\text{train}} > k$ , as  $n \rightarrow \infty$  we have

$$\begin{aligned} \tilde{\beta}_j &\rightarrow_p \text{Var}(X_{j,i})^{-1} \text{Cov}(X_{j,i}, \mu_{n_{\text{train}}}(\mathbf{X}_i, A_i)) \\ &= \text{Var}(X_{j,i})^{-1} \text{Cov}(X_{j,i}, \mu_{n_{\text{train}}}(\mathbf{X}_i, A_i) - \mu(\mathbf{X}_i, A_i) + \mu(\mathbf{X}_i, A_i)) \\ &= \text{Var}(X_{j,i})^{-1} \{ \text{Cov}(X_{j,i}, \mu_{n_{\text{train}}}(\mathbf{X}_i, A_i) - \mu(\mathbf{X}_i, A_i)) + \text{Cov}(X_{j,i}, \mu(\mathbf{X}_i, A_i)) \} \\ &\leq \text{Var}(X_{j,i})^{-1} \left\{ \sqrt{\text{Var}(X_{j,i}) \text{Var}(\mu_{n_{\text{train}}}(\mathbf{X}_i, A_i) - \mu(\mathbf{X}_i, A_i))} + \text{Cov}(X_{j,i}, \mu(\mathbf{X}_i, A_i)) \right\}, \end{aligned}$$

where the last line comes from the Cauchy–Schwarz inequality. Since  $E[(\mu_{n_{\text{train}}}(\mathbf{X}_i, A_i) - \mu(\mathbf{X}_i, A_i))^2] \rightarrow 0$  as  $n_{\text{train}} \rightarrow \infty$ , the square root term also approaches zero as  $n_{\text{train}} \rightarrow \infty$ . Thus, we have

$$\tilde{\beta}_j \rightarrow_p \text{Var}(X_{j,i})^{-1} \text{Cov}(X_{j,i}, \mu(\mathbf{X}_i, A_i)) \quad (\text{E.29})$$

as  $n, n_{\text{train}} \rightarrow \infty$ .

Since the right-hand side of Line (E.29) equals the right-hand side of Line (E.9), we have shown that  $\hat{\beta}_j$  and  $\tilde{\beta}_j$  still converge to a common limit as  $n, n_{\text{train}} \rightarrow \infty$ .

## F Proofs for Theorem 2 and associated results

### F.1 Proof of Theorem 2

*Proof.* Below, we prove the more general version of the result where, rather than assuming Condition 1, we assume that

$$E \left[ \hat{\Delta}_{\text{snoop}}(\mathbf{X}, \mathbf{U}^{(0)}) \right] + r \geq E \left[ \hat{\Delta}_{\text{snoop}}(\mathbf{X}, \mathbf{U}^{(1-\rho^2)}) \right] \quad (\text{F.1})$$

for some constant  $r \geq 0$  (see Section 2.2). Condition 1 is of course the special case where  $r = 0$ . Below, we will also address the special case where Eq (F.1) holds with equality. Without loss of generality (WLOG), we assume that  $\mathbf{Y}$  is shifted so that  $E[\mu(\mathbf{X}, \mathbf{0})] = 0$  (see Eq (D.1)).

We start by showing Eq (5). Conditioning on  $(\mathbf{x}, \mathbf{a})$  and applying Eq (3) gives

$$\begin{aligned}
& E_{\mathbf{Y}|\mathbf{x},\mathbf{a}}[\hat{\Delta}_{\text{blind}}(\mathbf{x}, \mathbf{Y})] \\
&= E_{\mathbf{Y}|\mathbf{x},\mathbf{a}}d(x_{j'}, \mathbf{Y}) \quad \text{where } j' = \arg \max_{j \in \{1, \dots, p\}} d(\mathbf{x}_j, \mu(\mathbf{x}, \mathbf{a})) \\
&= d(x_{j'}, E_{\mathbf{Y}|\mathbf{x},\mathbf{a}} \mathbf{Y}) \quad \text{from linearity of } d \\
&= d(x_{j'}, \mu(\mathbf{x}, \mathbf{a})) \\
&= \max_{j \in \{1, \dots, p\}} d(\mathbf{x}_j, \mu(\mathbf{x}, \mathbf{a})). \tag{F.2}
\end{aligned}$$

Iterating expectations then shows Eq (5):

$$\begin{aligned}
E_{\mathbf{X},\mathbf{A}} E_{\mathbf{Y}|\mathbf{X},\mathbf{A}}[\hat{\Delta}_{\text{blind}}(\mathbf{X}, \mathbf{Y})] &= E_{\mathbf{X},\mathbf{A}} \max_{j \in \{1, \dots, p\}} d(\mathbf{X}_j, \mu(\mathbf{X}, \mathbf{A})) \\
&= E_{\mathbf{X},\mathbf{A}} \hat{\Delta}_{\text{snoop}}(\mathbf{X}, \mu(\mathbf{X}, \mathbf{A})).
\end{aligned}$$

Next, we note that

$$\begin{aligned}
\rho^{-1} \mathbf{U}^{(1-\rho^2)} &= \rho^{-1} \left\{ \mu(\mathbf{X}, 0) \rho + \mathbf{U} \sqrt{1 - \rho^2} \right\} \\
&= \mu(\mathbf{X}, 0) + \mathbf{U} \sqrt{(1 - \rho^2) / \rho^2} \\
&= \mu(\mathbf{X}, 0) + \mathbf{U} \sqrt{\left( \frac{E[Var(Y_i - A_i \Delta | \mathbf{X}_i, A_i)]}{Var(Y_i - A_i \Delta)} \right) / \left( \frac{Var(\mu(\mathbf{X}_i, 0))}{Var(Y_i - A_i \Delta)} \right)} \\
&= \mu(\mathbf{X}, 0) + \mathbf{U} \sqrt{\frac{E[Var(\epsilon_i | \mathbf{X}_i, \mathbf{A}_i)]}{Var(\mu(\mathbf{X}_i, 0))}} \\
&= \mu(\mathbf{X}, 0) + \mathbf{U} \sqrt{\frac{Var(\epsilon_i)}{Var(U_i)}},
\end{aligned}$$

where the second term in the last line has the same variance as  $\epsilon$ . Centering this term gives

$$\rho^{-1} \mathbf{U}^{(1-\rho^2)} - E \left[ \mathbf{U} \sqrt{\frac{Var(\epsilon_i)}{Var(U_i)}} \right] = \mu(\mathbf{X}, 0) + (\mathbf{U} - E[\mathbf{U}]) \sqrt{\frac{Var(\epsilon_i)}{Var(U_i)}}, \tag{F.3}$$

Where the second term on the right-hand side of Eq (F.3) now has the same mean and variance as  $\epsilon$ , and therefore has the same distribution as  $\epsilon$  by Condition 4. Since  $\epsilon, \mathbf{U} \perp \mathbf{X}, \mathbf{A}$  (Condition 3), we see from Eq (F.3) that  $(\mathbf{A}, \mathbf{X}, \rho^{-1} \mathbf{U}^{(1-\rho^2)} - E[\mathbf{U} \sqrt{Var(\epsilon)/Var(U)}])$  follows the same joint distribution as  $(\mathbf{A}, \mathbf{X}, \mu(\mathbf{X}, 0) + \epsilon) = (\mathbf{A}, \mathbf{X}, \mathbf{Y} - \mathbf{A} \Delta)$ . Applying this in Line

(F.5), below, gives

$$\begin{aligned}
& E\hat{\Delta}_{\text{blind}}(\mathbf{X}, \mathbf{Y}) - \Delta \\
&= E \max_{j \in \{1, \dots, p\}} d(\mathbf{X}_j, \mu(\mathbf{X}, \mathbf{A})) - \Delta && \text{from Eq (5)} \\
&= E \max_{j \in \{1, \dots, p\}} d(\mathbf{X}_j, \mu(\mathbf{X}, \mathbf{0}) + A\Delta) - \Delta && \text{from Cond. 2} \\
&= E \max_{j \in \{1, \dots, p\}} d(\mathbf{X}_j, \mu(\mathbf{X}, \mathbf{0})) && \text{from Eq (D.2)} \\
&\geq E \max_{j \in \{1, \dots, p\}} d(\mathbf{X}_j, \mathbf{U}^{(1-\rho^2)}) - r && \text{from Eq (F.1)} \quad (\text{F.4}) \\
&= \rho E \max_{j \in \{1, \dots, p\}} d(\mathbf{X}_j, \mathbf{U}^{(1-\rho^2)} \rho^{-1}) - r && \text{from linearity} \\
&= \rho E \max_{j \in \{1, \dots, p\}} d \left( \mathbf{X}_j, \mathbf{U}^{(1-\rho^2)} \rho^{-1} - E \left[ \mathbf{U} \sqrt{\frac{\text{Var}(\epsilon)}{\text{Var}(U)}} \right] \right) - r && \text{from Eq (D.1)} \\
&= \rho E \max_{j \in \{1, \dots, p\}} d(\mathbf{X}_j, \mathbf{Y} - \mathbf{A}\Delta) - r && (\text{F.5}) \\
&= \rho \left( E \left[ \max_{j \in \{1, \dots, p\}} d(\mathbf{X}_j, \mathbf{Y}) \right] - \Delta \right) - r && \text{from Eq (D.2)} \\
&= \rho \left( E \left[ \hat{\Delta}_{\text{snoop}}(\mathbf{X}, \mathbf{Y}) \right] - \Delta - r\rho^{-1} \right). && (\text{F.6})
\end{aligned}$$

Above, Line (F.5) comes from the simple fact that, for any function  $f$ , we have  $Ef(\mathbf{Z}) = Ef(\mathbf{Z}')$  when  $\mathbf{Z}$  and  $\mathbf{Z}'$  have the same (multivariate) distribution.

If Eq (F.1) holds with equality, then Lines (F.4)-(F.6) also hold with equality.  $\square$

## F.2 Proof of Remark 10

We will assume WLOG that  $\text{Var}(X_j) = 1$  for all  $j$ , as the scale of  $\mathbf{X}_j$  does not affect the estimate  $d(\mathbf{X}_j, \mathbf{Y})$ . Let  $k_j^{(m)} = \text{Cov}(\mathbf{U}^{(m)}, \mathbf{X}_j)$ , let  $\sigma_\mu^2 = \text{Var}(\mu(\mathbf{X}, \mathbf{A}))$ , and recall that  $\mathbf{U}^{(m)}$  is defined as  $\mu(\mathbf{X}, 0) \sqrt{1-m} + \mathbf{U} \sqrt{m}$ .

First, we write  $d_0(\mathbf{X}_j, \mathbf{U}^{(m)})$  as a difference in means.

$$\begin{aligned}
d_0(\mathbf{X}_j, \mathbf{U}^{(m)}) &= \arg \min_{b_a} \left[ \min_{b_0} \left\| \mathbf{U}^{(m)} - \left( b_0 + X_j k_j^{(m)} + b_a \mathbf{A} \right) \right\|_2^2 \right] \\
&= \sum_{i=1}^n \left\{ \left( \frac{A_i}{\mathbf{1}^\top \mathbf{A}} - \frac{(1-A_i)}{n - \mathbf{1}^\top \mathbf{A}} \right) \left( U_i^{(m)} - X_{j,i} k_j^{(m)} \right) \right\}.
\end{aligned}$$

Since  $\mathbf{A} \perp \mathbf{X}$ , this difference has expectation zero, given  $\mathbf{A}$ . That is,  $E[d_0(\mathbf{X}_j, \mathbf{U}^{(m)}) | \mathbf{A}] = 0$ .

For any two indices  $j, j'$ , the law of total covariance tells us that

$$\begin{aligned}
& Cov(d_0(\mathbf{X}_j, \mathbf{U}^{(m)}), d_0(\mathbf{X}_{j'}, \mathbf{U}^{(m)})) \\
&= E[Cov(d_0(\mathbf{X}_j, \mathbf{U}^{(m)}), d_0(\mathbf{X}_{j'}, \mathbf{U}^{(m)})|A)] + Cov(E[d_0(\mathbf{X}_j, \mathbf{U}^{(m)})|A], E[d_0(\mathbf{X}_{j'}, \mathbf{U}^{(m)})|A]) \\
&= E[Cov(d_0(\mathbf{X}_j, \mathbf{U}^{(m)}), d_0(\mathbf{X}_{j'}, \mathbf{U}^{(m)})|A)] + 0 \\
&= \sum_{i=1}^n E\left[\left(\frac{A_i}{\mathbf{1}^\top \mathbf{A}} - \frac{(1-A_i)}{n - \mathbf{1}^\top \mathbf{A}}\right)^2\right] Cov(U_i^{(m)} - X_{j,i}k_1^{(m)}, U_i^{(m)} - X_{j',i}k_2^{(m)}) \\
&\propto Cov(U_i^{(m)} - X_{j,i}k_j^{(m)}, U_i^{(m)} - X_{j',i}k_{j'}^{(m)}) \\
&= Cov(U_i^{(m)}, U_i^{(m)}) - k_j^{(m)}Cov(U_i^{(m)}, X_{j,i}) - k_{j'}^{(m)}Cov(U_i^{(m)}, X_{j',i}) + k_j^{(m)}k_{j'}^{(m)}Cov(X_{j,i}, X_{j',i}) \\
&= \sigma_\mu^2 - \left(k_j^{(m)}\right)^2 - \left(k_{j'}^{(m)}\right)^2 + k_j^{(m)}k_{j'}^{(m)}\rho_{j,j'}. \tag{F.7}
\end{aligned}$$

We can replace  $k_j^{(m)}$  by noting that

$$k_j^{(m)} = Cov(\mathbf{U}^{(m)}, \mathbf{X}_j) = Cov(\mu(\mathbf{X}, \mathbf{0}), \mathbf{X}_j) \sqrt{1-m} = \sigma_\mu \rho_{\mu,j} \sqrt{1-m}.$$

Plugging this into Eq (F.7) gives

$$\begin{aligned}
& Cov(d_0(\mathbf{X}_j, \mathbf{U}^{(m)}), d_0(\mathbf{X}_{j'}, \mathbf{U}^{(m)})) \\
&\propto \sigma_\mu^2 + (1-m)(-\sigma_\mu^2 \rho_{\mu,j}^2 - \sigma_\mu^2 \rho_{\mu,j'}^2 + \sigma_\mu^2 \rho_{\mu,j} \rho_{\mu,j'} \rho_{j,j'}) \\
&\propto 1 + (1-m)(-\rho_{\mu,j}^2 - \rho_{\mu,j'}^2 + \rho_{\mu,j} \rho_{\mu,j'} \rho_{j,j'}) \\
&= 1 + (1-m)b_{jj'},
\end{aligned}$$

and

$$Cor(d(\mathbf{X}_1, \mathbf{U}^{(m)}), d(\mathbf{X}_2, \mathbf{U}^{(m)})) = \frac{1 + (1-m)b_{12}}{\sqrt{1 + (1-m)b_{11}} \sqrt{1 + (1-m)b_{22}}}.$$

### F.3 Proof of Corollaries 4 & 5

*Proof.* Again, we will prove the more general result, replacing Condition 1 of Theorem 2 with Eq (F.1).

For Corollary 4, we note that the relation in Theorem 2 holds for any fixed  $\mathcal{S}$ , as the proof steps in Section F.1 are unchanged if we replace the  $\max_{j \in \{1, \dots, p\}}$  operator with  $\max_{j \in \mathcal{S}}$ , and replace  $\hat{\Delta}_{\text{snoop}}$  and  $\hat{\Delta}_{\text{blind}}$  with  $\hat{\Delta}_{\text{snoop}, \mathcal{S}}$  and  $\hat{\Delta}_{\text{blind}, \mathcal{S}}$  respectively. Iterating expectations then yields

$$\begin{aligned}
E[\hat{\Delta}_{\text{blind}, \mathcal{S}}(\mathbf{X}, \mathbf{Y})] - \Delta &= E_{\mathcal{S}} E[\hat{\Delta}_{\text{blind}, \mathcal{S}'}(\mathbf{X}, \mathbf{Y}) - \Delta | \mathcal{S} = \mathcal{S}'] \\
&\geq \rho E_{\mathcal{S}} E[\hat{\Delta}_{\text{snoop}, \mathcal{S}'}(\mathbf{X}, \mathbf{Y}) - \Delta - r\rho^{-1} | \mathcal{S} = \mathcal{S}'] \\
&= \rho(E\hat{\Delta}_{\text{snoop}, \mathcal{S}}(\mathbf{X}, \mathbf{Y}) - \Delta - r\rho^{-1}).
\end{aligned}$$

Similarly, for Corollary 5, we note that the steps in Section F.1 are unchanged if we replace the  $\max_{j \in \{1, \dots, p\}} d(\mathbf{X}_j, \mathbf{z})$  with  $d_{(c)}(\mathbf{X}, z)$  for any  $z \in \mathbb{R}^n$ , and replace  $\hat{\Delta}_{\text{snoop}}$  and  $\hat{\Delta}_{\text{blind}}$  with  $\hat{\Delta}_{\text{snoop}, c}$  and  $\hat{\Delta}_{\text{blind}, c}$  respectively. Iterating expectations now gives the result.

$$\begin{aligned} E\hat{\Delta}_{\text{blind}, C}(\mathbf{X}, \mathbf{Y}) - \Delta &= E_C \left[ E \left( \hat{\Delta}_{\text{blind}, C}(\mathbf{X}, \mathbf{Y}) - \Delta | C \right) \right] \\ &\geq E_C \left[ \rho \left\{ E \left( \hat{\Delta}_{\text{snoop}, C}(\mathbf{X}, \mathbf{Y}) | C \right) - \Delta - r\rho^{-1} \right\} \right] \\ &= \rho \left\{ E \left( \hat{\Delta}_{\text{snoop}, C}(\mathbf{X}, \mathbf{Y}) \right) - \Delta - r\rho^{-1} \right\}. \end{aligned}$$

□

## G Proof of Remark 8

*Proof.* Let  $C$  be a random variable such that  $f_C \in \mathcal{F}$  is the randomly selected function from Step 2 of Algorithm 7, and  $C \perp \{Y_i, \mathbf{X}_i, A_i\}_{\{i \notin \mathcal{I}_1^{\text{treat}}\}}$ . Let  $c$  denote realizations of  $C$ . Regardless of the marginal distribution of  $C$ , we have

$$\begin{aligned} &E \left[ \left( \frac{\sum_{i=1}^n Y_i A_i}{\sum_{i=1}^n A_i} \right) - f_C(\{Y_i, \mathbf{X}_i, A_i\}_{\{i \notin \mathcal{I}_1^{\text{treat}}\}}) \right] \\ &= E \left( \frac{\sum_{i=1}^n Y_i A_i}{\sum_{i=1}^n A_i} \right) - E[f_C(\{Y_i, \mathbf{X}_i, A_i\}_{\{i \notin \mathcal{I}_1^{\text{treat}}\}})] \\ &= E(Y_i | A_i = 1) - E_C[E\{f_c(\{Y_i, \mathbf{X}_i, A_i\}_{\{i \notin \mathcal{I}_1^{\text{treat}}\}}) | C = c\}] \\ &= E(Y_i | A_i = 1) - E_C[E\{f_c(\{Y_i, \mathbf{X}_i, A_i\}_{\{i \notin \mathcal{I}_1^{\text{treat}}\}})\}] \tag{G.1} \\ &= E(Y_i | A_i = 1) - E_C[E(\tilde{Y}_i^{\text{control}} | A_i = 1)] \\ &= E(\tilde{Y}_i^{\text{treat}} | A_i = 1) - E(\tilde{Y}_i^{\text{control}} | A_i = 1). \end{aligned}$$

Above, Line (G.1) comes from the assumption that  $C \perp \{Y_i, \mathbf{X}_i, A_i\}_{\{i \notin \mathcal{I}_1^{\text{treat}}\}}$ . □

## H Proof of Theorem B.1

We proceed in two steps. In Section H.1, we derive the categorical variable that creates the highest possible snooping bias, and the categorical variable that creates the highest possible blinded bias. In Sections H.2 & H.3, we evaluate these two biases, and reduce them to the right-hand sides of Eqs (B.1) & (B.2) respectively.

Throughout this proof we will use notation for arm-specific order statistics. Let  $Z_{(a,i)}$  denote the  $i^{\text{th}}$  order statistic for a random variable  $\mathbf{Z}$  within arm  $a$ . This means, for example, that  $Y_{(1,1)} \leq \dots \leq Y_{(1,n/2)}$  with  $\{Y_{(1,1)}, \dots, Y_{(1,n/2)}\} = \{Y_i : A_i = 1\}$ ; and that  $\mu(\mathbf{X}, \mathbf{A})_{(0,1)} \leq \dots \leq \mu(\mathbf{X}, \mathbf{A})_{(0,n/2)}$  with  $\{\mu(\mathbf{X}, \mathbf{A})_{(0,1)}, \dots, \mu(\mathbf{X}, \mathbf{A})_{(0,n/2)}\} = \{\mu(\mathbf{X}_i, A_i) : A_i = 0\}$ .

In general, we will assume below that analysts can adaptively define any binary covariate they wish. In this case, we will see that the bounds in Theorem B.1 hold with equality. Alternatively, in the  $p \rightarrow \infty$  setting described in Theorem B.1, the probability that one of

the observed covariates will equal the “worst-case” covariate (i.e., a covariate taking values equal to what the analysts would have chosen adaptively, if given the opportunity) slowly approaches 1.

## H.1 Preliminaries: worst-case features in unblinded and blinded settings

In this section we introduce two lemmas that describe the worst possible (discrete) variables that analysts can to adjust for.

For the blinded setting, bias can occur when researchers stratify on apparent risk factors that are, by chance, rare on control and common on treatment. In the extreme, we will see below that the binary vector  $\mathbf{x}'$  satisfying the following condition will produce the IPW estimate with the worst possible bias.

**Condition H.1.** (Worst-case unblinded features) Given the observed values of  $\mathbf{y}$  and  $\mathbf{a}$ , where  $a_i = 0$  if and only if  $i \leq n/2$ , the discrete feature vector  $\mathbf{x}' \in \mathbb{R}^n$  satisfies

- (Include lowest control)  $x'_i = 1$  for any value  $i$  in the set  $\{i : a_i = 0 \text{ and } y_i = y_{(0,1)}\}$ ;
- (Exclude remaining controls)  $x'_i = 0$  for any value  $i$  in the set  $\{i : a_i = 0 \text{ and } y_i > y_{(0,1)}\}$ ;
- (Exclude highest treated)  $x'_i = 0$  for any value  $i$  in the set  $\{i : a_i = 1 \text{ and } y_i = y_{(1,n/2)}\}$ ; and
- (Include remaining treated)  $x'_i = 1$  for any value  $i$  in the set  $\{i : a_i = 1 \text{ and } y_i < y_{(1,n/2)}\}$ .

Figure B.1 shows an example of a feature that satisfies Condition H.1. In words, Condition H.1 requires that  $\mathbf{x}'$  is 1 only for the control observation with the lowest outcome, and is zero for all other controls. Within treated, Condition H.1 requires that  $\mathbf{x}'$  equals 1 for everyone except the person with the highest outcome. As  $\mathbf{X}$  contains a random variable  $\mathbf{X}_j$  that is continuous, a malicious analyst can almost always adaptively define a feature  $\mathbf{x}'$  that satisfies Condition H.1 (with probability 1) by defining  $\mathbf{x}'$  as a function of  $\mathbf{x}_j$ .

The next lemma (proved below, in Section H.1.1) states that adjusting for any feature satisfying Condition H.1 does indeed produce the worst possible bias.

**Lemma H.2.** (Worst-case added variable bias) *If  $n$  is an even number no less than 4, and  $a_i = 1(i > n/2)$ , then any feature  $\mathbf{x}'$  satisfying Condition H.1 in a particular dataset  $\{\mathbf{y}, \mathbf{x}\}$  produces the highest value of  $d_{IPW}(\mathbf{x}', \mathbf{y})$  for that dataset, over all discrete features.*

The intuition behind Lemma H.2 is that balancing on any other feature will only shift weight away from the extremes of the sample.

Similarly, we can put forward a version of Condition H.1 where the blinded outcomes  $\mathbf{Y}$  are replaced with their observed proxies,  $\mu(\mathbf{X}, \mathbf{A})$ .

**Condition H.3.** (Blinded version of Condition H.1) Given the observed, blinded datasets  $\{\mathbf{x}, \mathbf{a}\}$  and predicted outcomes  $\mu(\mathbf{x}, \mathbf{a})$ , the feature  $\mathbf{x}'$  satisfies

- (Include lowest control)  $x'_i = 1$  for any value  $i$  in the set  $\{i : a_i = 0 \text{ and } \mu(\mathbf{x}_i, a_i) = \mu(\mathbf{x}, \mathbf{a})_{(0,1)}\}$ ;

- (Exclude remaining controls)  $x'_i = 0$  for any value  $i$  in the set  $\{i : a_i = 0 \text{ and } \mu(\mathbf{x}_i, a_i) > \mu(\mathbf{x}, \mathbf{a})_{(0,1)}\}$ ;
- (Exclude highest treated)  $x'_i = 0$  for any value  $i$  in the set  $\{i : a_i = 1 \text{ and } \mu(\mathbf{x}_i, a_i) = \mu(\mathbf{x}, \mathbf{a})_{(1,n/2)}\}$ ;  
and
- (Include remaining treated)  $x'_i = 1$  for any value  $i$  in the set  $\{i : a_i = 1 \text{ and } \mu(\mathbf{x}_i, a_i) < \mu(\mathbf{x}, \mathbf{a})_{(1,n/2)}\}$ .

Analogous to Condition H.1, Condition H.3 represents the extreme case of a risk factor that is, by chance, rare on control and common on treatment. Weighting on a feature  $\mathbf{x}'$  that satisfies Condition H.3 will upweight treated patients with outcomes that are expected to be high, and upweight control patients with outcomes that are expected to be low. As with Condition H.1, a malicious analyst can almost always satisfy Condition H.3 (with probability 1) if one of the covariates is continuous.

Finally, we note that a variable satisfying Condition H.3 does indeed produce the worst possible bias for a blinded analyst.

**Lemma H.4.** (*Blinded version of Lemma H.2*) Suppose that  $n$  is an even number no less than 4; that  $a_i = 1 (i > n/2)$ ; and that the covariates  $\mathbf{X}$  and treatments  $a$  are observed by a blinded analyst, but the outcomes  $y$  are not. Given the observed covariates  $\mathbf{x}$ , balancing on a feature  $\mathbf{x}'$  satisfying Condition H.3 produces the highest possible value of  $E[d_{IPW}(\mathbf{x}', \mathbf{Y})|\mathbf{x}, \mathbf{a}]$  over all discrete features.

The proof follows the same logic as the proof for Lemma H.2, but with predicted outcomes replacing the observed outcomes (see Section H.1.1).

### H.1.1 Proof of Lemmas H.2 & H.4

*Proof.* Since  $d_{IPW}(\mathbf{x}_j, \mathbf{y})$  is set to zero whenever one of the categories of  $\mathbf{x}_j$  is empty on treatment or control, we only consider categorical variables that have at least one treated and control observation in each category.

We first note that any inverse propensity weight  $(\pi(k; \hat{a}_j))^{-1}$ , where  $k$  is the realization of a categorical variable) must be between  $n/2$  and  $\frac{n/2}{n/2-1}$ . To see this, let  $t_k := \sum_{i=1}^n a_i 1(x_i = k)$  and  $c_k := \sum_{i=1}^n (1 - a_i) 1(x_i = k)$  be the number of treated and control patients in the  $k^{\text{th}}$  group. Since each  $\mathbf{X}_j$  is discrete, and there is at least one treated and control observation in each category, we have  $c_k, t_k \in [1, n/2 - 1]$  and  $\pi(k, \hat{a}_j) = \frac{t_k}{t_k + c_k}$ . We can now see that the maximum IPW weight is no more than

$$\begin{aligned} \max_{c_k, t_k \in [1, n/2-1]} \left( \frac{t_k}{t_k + c_k} \right)^{-1} &= \max_{c_k, t_k \in [1, n/2-1]} 1 + c_k/t_k \\ &= n/2. \end{aligned}$$

Likewise, the smallest possible IPW weight is no less than

$$\begin{aligned} \min_{c_k, t_k \in [1, n/2-1]} \left( \frac{t_k}{t_k + c_k} \right)^{-1} &= \min_{c_k, t_k \in [1, n/2-1]} 1 + c_k/t_k \\ &= 1 + \frac{1}{n/2 - 1} \\ &= \frac{n/2}{n/2 - 1}. \end{aligned}$$

From here, we show Lemma H.2 by noting that the realization of Eq (H.3) assigns maximal weight to  $y_{(0,1)}$  and  $y_{(1,n/2)}$ , and minimal weight to the remaining observations. Our effect estimate is equal to a difference of two weighted means, one for each arm (see Eq (1)). The weighted mean within the treated arm is a convex combination of the observations in that arm. Thus, any deviation from the weights in Eq (H.3) must involve shifting weight towards lower outcomes  $y_i$  on treatment, which would reduce the estimated treatment effect. Likewise, any change to the control weights must result in shifting weight towards higher outcomes  $y_i$  on control, which would also reduce the estimated treatment effect. This completes the proof of Lemma H.2.

The proof for Lemma H.4 is similar, but replaces  $y_i$  with  $\mu(\mathbf{x}_i, a_i)$ . Given  $\mathbf{x}, \mathbf{a}$ , the conditional expectation of  $d_{\text{IPW}}(\mathbf{x}, \mathbf{Y})$  is

$$\frac{\sum_{i=1}^n \mu(x_i, a_i) a_i \pi(x_{j,i}; \hat{\alpha}_j)^{-1}}{\sum_{i=1}^n a_i \pi(x_{j,i}; \hat{\alpha}_j)^{-1}} - \frac{\sum_{i=1}^n \mu(x_i, a_i) (1 - a_i) (1 - \pi(x_{j,i}; \hat{\alpha}_j))^{-1}}{\sum_{i=1}^n (1 - a_i) (1 - \pi(x_{j,i}; \hat{\alpha}_j))^{-1}}.$$

As before, we know that  $d_{\text{IPW}}(\mathbf{x}, \mathbf{Y})$  places maximal weight on  $\mu(\mathbf{x}, \mathbf{a})_{(1,n/2)}$  and  $\mu(\mathbf{x}, \mathbf{a})_{(0,1)}$ , and minimal weight on the remaining terms. Any other weighting scheme will either shift weight towards lower values in  $\mu(\mathbf{x}, \mathbf{a})$  that are associated with the treatment arm, or shift weight towards higher values in  $\mu(\mathbf{x}, \mathbf{a})$  that are associated with the control arm. Either of these changes will diminish the conditional expectation of the effect estimate.  $\square$

## H.2 Proof of Eq (B.1)

*Proof.* Since each  $\mathbf{X}_j$  is discrete, we have  $\pi(k, \hat{\alpha}_j) = \frac{\sum_{i=1}^n a_i 1(x_{j,i}=k)}{\sum_{i=1}^n 1(x_{j,i}=k)}$ , and

$$\begin{aligned} \sum_{i=1}^n a_i \pi(x_{j,i}; \hat{\alpha}_j)^{-1} &= \sum_{k=1}^K \sum_{i'=1}^n a_{i'} 1(x_{j,i'} = k) \pi(k; \hat{\alpha}_j)^{-1} \\ &= \sum_{k=1}^K \frac{\sum_{i'=1}^n a_{i'} 1(x_{j,i'} = k) \sum_{i=1}^n 1(x_{j,i} = k)}{\sum_{i=1}^n a_i 1(x_{j,i} = k)} \\ &= \sum_{k=1}^K \sum_{i=1}^n 1(x_{j,i} = k) \\ &= n \end{aligned}$$

for all  $j$ . Likewise,  $1 - \pi(k, \hat{\alpha}_j) = \frac{\sum_{i=1}^n (1 - a_i) 1(x_{j,i}=k)}{\sum_{i=1}^n 1(x_{j,i}=k)}$ , and  $\sum_{i=1}^n (1 - a_i) (1 - \pi(x_{j,i}; \hat{\alpha}_j))^{-1} = n$  for all  $j$ .

If  $\mathbf{X}_{j^\dagger}$  is chosen adaptively to satisfy Condition H.1, and all values of  $Y_i$  are distinct, we have  $\hat{\pi}(0, \alpha_{j^\dagger}) = 1/(n/2)$  and  $\pi(1, \alpha_{j^\dagger}) = \{(n/2) - 1\}/(n/2)$ . Since the only influence of  $\mathbf{X}_{j^\dagger}$  is in determining propensity score weights, we can effectively view these weights as fixed – in any sample we can find an  $\mathbf{X}_{j^\dagger}$  that produces the same weights. Condition H.1 also tells us that

$$\begin{aligned}
d_{\text{IPW}}(\mathbf{X}_{j^\dagger}, \mathbf{Y}) &= \frac{\sum_{i=1}^n Y_i a_i \pi(X_{j^\dagger, i}; \hat{\alpha}_{j^\dagger})^{-1}}{\sum_{i=1}^n a_i \pi(X_{j^\dagger, i}; \hat{\alpha}_{j^\dagger})^{-1}} - \frac{\sum_{i=1}^n y_i (1 - a_i) (1 - \pi(X_{j^\dagger, i}; \hat{\alpha}_{j^\dagger}))^{-1}}{\sum_{i=1}^n (1 - a_i) (1 - \pi(X_{j^\dagger, i}; \hat{\alpha}_{j^\dagger}))^{-1}} \\
&= \sum_{i=1}^n \frac{Y_i a_i}{n \pi(X_{j^\dagger, i}; \hat{\alpha}_{j^\dagger})} - \frac{\sum_{i=1}^n y_i (1 - a_i)}{n (1 - \pi(X_{j^\dagger, i}; \hat{\alpha}_{j^\dagger}))} \tag{H.1}
\end{aligned}$$

$$\begin{aligned}
&= \sum_{\{i: x'_i=0\}} \left[ \frac{a_i Y_i}{n \pi(X_{j^\dagger, i}; \hat{\alpha}_{j^\dagger})} - \frac{(1 - a_i) Y_i}{n (1 - \pi(X_{j^\dagger, i}; \hat{\alpha}_{j^\dagger}))} \right] \\
&\quad + \sum_{\{i: x'_i=1\}} \left[ \frac{a_i Y_i}{n \pi(X_{j^\dagger, i}; \hat{\alpha}_{j^\dagger})} - \frac{(1 - a_i) Y_i}{n (1 - \pi(X_{j^\dagger, i}; \hat{\alpha}_{j^\dagger}))} \right] \tag{H.2}
\end{aligned}$$

$$\begin{aligned}
&= \frac{Y_{(1, n/2)}}{n \pi(0; \hat{\alpha}_{j^\dagger})} - \frac{\sum_{i=2}^{n/2} Y_{(0, 1)}}{n (1 - \pi(0; \hat{\alpha}_{j^\dagger}))} + \frac{\sum_{i=1}^{(n/2)-1} Y_{(1, i)}}{n \pi(1; \hat{\alpha}_{j^\dagger})} - \frac{Y_{(0, 1)}}{n (1 - \pi(1; \hat{\alpha}_{j^\dagger}))} \quad \text{by Condition H.1} \\
&= \frac{Y_{(1, n/2)}}{2} - \frac{\sum_{i=2}^{n/2} Y_{(0, 1)}}{n - 2} + \frac{\sum_{i=1}^{(n/2)-1} Y_{(1, i)}}{n - 2} - \frac{Y_{(0, 1)}}{2} \\
&= \frac{Y_{(1, n/2)} - Y_{(0, 1)}}{2} + \left\{ \frac{\sum_{j=1}^{(n/2)-1} Y_{(1, j)}}{n - 2} - \frac{\sum_{i=2}^{(n/2)} Y_{(0, i)}}{n - 2} \right\} \\
&= \frac{Y_{(1, n/2)} - Y_{(0, 1)}}{2} + \left\{ \frac{\sum_{i=2}^{(n/2)-1} Y_{(1, i)} - Y_{(0, i)}}{n - 2} \right\} + \frac{Y_{(1, 1)} - Y_{(0, n/2)}}{n - 2}. \tag{H.3}
\end{aligned}$$

Since  $\tilde{Y}^{\text{treat}} = \tilde{Y}^{\text{control}} + \Delta$ , we know that  $E[\tilde{Y}_{(1, i)}^{\text{treat}}] = E[\tilde{Y}_{(0, i)}^{\text{control}}] + \Delta$  for any  $i$ . From our assumptions, we also know that  $Y_i$  follows the same marginal distribution as  $\tilde{Y}_i^{\text{treat}}$  when  $A_i = 1$ , and  $Y_i$  follows the same distribution as  $\tilde{Y}_i^{\text{control}}$  when  $A_i = 0$ . It follows that,  $E[Y_{(1, i)}] = E[Y_{(0, i)}] + \Delta$ . Applying this to Eq (H.3), we have

$$\begin{aligned}
E[d_{\text{IPW}}(\mathbf{X}_j, \mathbf{Y})] &= \frac{\Delta + E\{Y_{(0, n/2)} - Y_{(0, 1)}\}}{2} + \left\{ \frac{\sum_{i=2}^{(n/2)-1} \Delta}{n - 2} \right\} + \frac{\Delta + E\{Y_{(0, 1)} - Y_{(0, n/2)}\}}{n - 2} \\
&= E\{Y_{(0, n/2)} - Y_{(0, 1)}\} \left( \frac{1}{2} - \frac{1}{n - 2} \right) + \Delta \left( \frac{1}{2} + \frac{n/2 - 2}{n - 2} + \frac{1}{n - 2} \right) \\
&= E\{Y_{(0, n/2)} - Y_{(0, 1)}\} \left( \frac{1}{2} - \frac{1}{n - 2} \right) + \Delta. \tag{H.4}
\end{aligned}$$

Combined with Lemma H.2, this proves the result.  $\square$

### H.3 Proof of Eq (B.2)

*Proof.* The proof for (B.2) follows similar steps as the proof for Eq (B.1), with  $\mathbf{Y}$  replaced with  $\mu(\mathbf{X}, \mathbf{A})$ . If  $\mathbf{X}_{j^\dagger}$  is chosen adaptively to satisfy Condition H.3, and all values of  $\mu(\mathbf{X}, \mathbf{A})$

are distinct, we again have  $\pi(0; \hat{\alpha}_{j^\dagger}) = 1/(n/2)$ ;  $\pi(1; \hat{\alpha}_{j^\dagger}) = \{(n/2) - 1\}/(n/2)$ ; and

$$d_{\text{IPW}}(\mathbf{X}_{j^\dagger}, \mu(\mathbf{X}, \mathbf{A})) = \frac{\mu(\mathbf{X}, \mathbf{A})_{(1, n/2)} - \mu(\mathbf{X}, \mathbf{A})_{(0, 1)}}{2} + \left\{ \frac{\sum_{i=2}^{(n/2)-1} \mu(\mathbf{X}, \mathbf{A})_{(1, i)} - \mu(\mathbf{X}, \mathbf{A})_{(0, i)}}{n-2} \right\} \\ + \frac{\mu(\mathbf{X}, \mathbf{A})_{(1, 1)} - \mu(\mathbf{X}, \mathbf{A})_{(0, n/2)}}{n-2}, \quad (\text{H.5})$$

from the same steps as in Eq (H.3).

We know from our assumptions that  $Y_i$  follows the same marginal distribution as  $\tilde{Y}_i^{\text{treat}}$  when  $A_i = 1$ ; that  $Y_i$  follows the same distribution as  $\tilde{Y}_i^{\text{control}}$  when  $A_i = 0$ ; and that  $\tilde{Y}^{\text{treat}} = \tilde{Y}^{\text{control}} + \Delta$ . It follows that  $\mu(\mathbf{x}, \mathbf{1}) = \mu(\mathbf{x}, \mathbf{0}) + \Delta$  for any  $\mathbf{x}$ , where  $\mathbf{1}$  and  $\mathbf{0}$  are  $n$ -length vectors of ones and zeros respectively. Thus,  $E[\mu(\mathbf{X}, \mathbf{1})_{(1, i)}] = E[\mu(\mathbf{X}, \mathbf{0})_{(0, i)}] + \Delta$  for any  $i$ . Since  $\{\mathbf{X}_i\}_{i=1}^n$  are *iid*, and  $\mathbf{A} \perp \mathbf{X}$ , we have

$$E[\mu(\mathbf{X}, \mathbf{A})_{(1, i)}] = E[\mu(\mathbf{X}, \mathbf{A})_{(0, i)}] + \Delta. \quad (\text{H.6})$$

Finally, Eqs (H.5) & (H.6) then tell us that

$$E[d_{\text{IPW}}(\mathbf{X}_{j^\dagger}, \mathbf{Y})] = E_{\mathbf{X}, \mathbf{A}} \{E[d_{\text{IPW}}(\mathbf{X}_{j^\dagger}, \mathbf{Y}) | \mathbf{X}, \mathbf{A}]\} \\ = E_{\mathbf{X}, \mathbf{A}} \{d_{\text{IPW}}(\mathbf{X}_{j^\dagger}, E[\mathbf{Y} | \mathbf{X}, \mathbf{A}])\} \\ = E_{\mathbf{X}, \mathbf{A}} \{d_{\text{IPW}}(\mathbf{X}_{j^\dagger}, \mu(\mathbf{X}, \mathbf{A}))\} \\ = \frac{\Delta + E[\mu(\mathbf{X}, \mathbf{A})_{(0, n/2)}] - E[\mu(\mathbf{X}, \mathbf{A})_{(0, 1)}]}{2} + \left\{ \frac{\sum_{i=2}^{(n/2)-1} \Delta}{n-2} \right\} \\ + \frac{\Delta + E[\mu(\mathbf{X}, \mathbf{A})_{(0, 1)}] - E[\mu(\mathbf{X}, \mathbf{A})_{(0, n/2)}]}{n-2} \\ = \{E[\mu(\mathbf{X}, \mathbf{A})_{(0, n/2)}] - E[\mu(\mathbf{X}, \mathbf{A})_{(0, 1)}]\} \left( \frac{1}{2} - \frac{1}{n-2} \right) + \Delta.$$

This, in combination with Lemma H.4, proves the result.  $\square$

## References

- Leadbetter, M. R., Lindgren, G., and Rootzén, H. (1983). *Extremes and related properties of random sequences and processes*. Springer, Berlin.
- Seber, G. A. and Lee, A. J. (2003). *Linear Regression Analysis, Second Edition*. John Wiley & Sons.
